# Supplementary material for: Learning Interaction-aware Guidance Policies for Motion Planning in Dense Traffic Scenarios
Source: arXiv:2107.04538 source file (2021-07-09)
Supplement: Supplementary file 1 [file appendix.tex]

\subsubsection{Training procedure}

\begin{figure}
\centering
\includegraphics[scale=0.33]{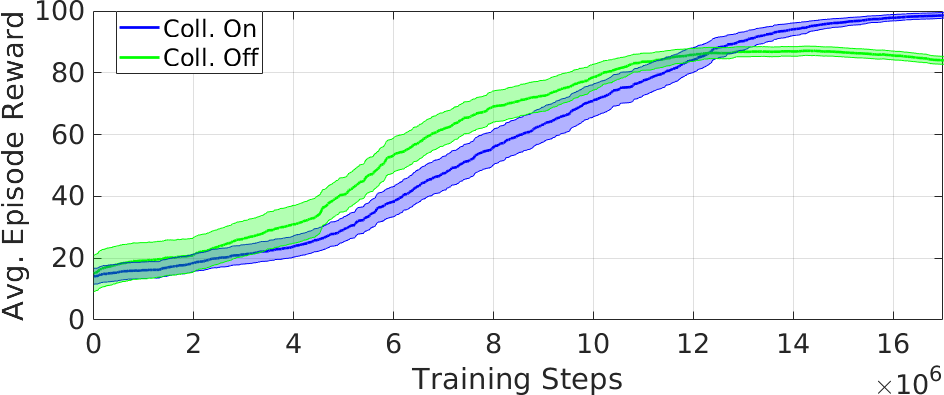}

\caption{Training evolution: Comparison of moving average rewards for a policy trained with collision constraints (Coll. On), depicted in blue, and without collision constraints (Coll. Off), depicted in green. Lines denote mean values and shaded areas around the lines denote standard deviations.}
\label{fig:training_evoluation}
\end{figure}

\begin{table*}[!t]
  \caption{ Evaluation of the impact of employing collision avoidance constraints on the learned policy's performance. Results are aggregated over 200 runs for each scenario (\cref{sec:driving_scenarios}) and each vehicle setting (\cref{sec:scenarios}). Both policies were trained considering a mixed setting for the other vehicles.}
         \centering
\begin{tabular}{c|c|c|c|c|c|c|c|c|c}
\hline
\multicolumn{1}{|c||}{}                 & \multicolumn{3}{|c||}{Cooperative} & \multicolumn{3}{c||}{Mixed} &
\multicolumn{3}{c|}{Non Cooperative} \\  \hline

\multicolumn{1}{|c||}{} &
\multicolumn{1}{c|}{Success(\%)} & \multicolumn{1}{c|}{Collision(\%)} &
\multicolumn{1}{c||}{Timeout(\%)} &
%\multicolumn{1}{c||}{Time(s)} &
\multicolumn{1}{c|}{Success(\%)} &
\multicolumn{1}{c|}{Collision(\%)} &
\multicolumn{1}{c||}{Timeout(\%)} &
%\multicolumn{1}{c||}{Time(s)} &
\multicolumn{1}{c|}{Success(\%)} &
\multicolumn{1}{c|}{Collision(\%)} &
\multicolumn{1}{c|}{Timeout(\%)} \\ \hline \hline %\multicolumn{1}{c|}{Time(s)} \\  \hline \hline

\multicolumn{1}{|c||}{\textit{Coll. On.}} &
\multicolumn{1}{c|}{\textbf{95.0}} &
\multicolumn{1}{c|}{0.0} &
\multicolumn{1}{c||}{\textbf{5.0}} &
%\multicolumn{1}{c||}{\textbf{34.3}} &
\multicolumn{1}{c|}{\textbf{91.0}} & 
\multicolumn{1}{c|}{0.0} &
\multicolumn{1}{c||}{\textbf{9.0}} &
%\multicolumn{1}{c||}{\textbf{35.5}} &
\multicolumn{1}{c|}{\textbf{36.0}} & 
\multicolumn{1}{c|}{0.0} &
\multicolumn{1}{c|}{\textbf{64.0}} \\ \hline
%\multicolumn{1}{c|}{-} \\  \hline

\multicolumn{1}{|c||}{\textit{Coll. Off}} & 
\multicolumn{1}{c|}{86.0} & 
\multicolumn{1}{c|}{0.0} &
\multicolumn{1}{c||}{14.0} &
%\multicolumn{1}{c||}{39.1} &
\multicolumn{1}{c|}{70.0} & 
\multicolumn{1}{c|}{0.0} &
\multicolumn{1}{c||}{30.0} &
%\multicolumn{1}{c||}{41.7} &
\multicolumn{1}{c|}{33.0} &
\multicolumn{1}{c|}{0.0} &
\multicolumn{1}{c|}{67.0} \\ \hline
%\multicolumn{1}{c|}{\textbf{45.5}} \\  \hline
\end{tabular}
\label{tab:ablation_coll_avd}
\end{table*}

We propose to jointly train the RL policy with the local optimization-based controller (\cref{alg:training}) allowing to directly deploy the trained policy on a real system. During training, employing collision constraints highly influences the close interaction of the AV with the other vehicles. Hence, we have trained two policies using \cref{alg:training} with collision constraints, denoted by \textit{Coll. On}, and without collision constraints, denoted by \textit{Coll. Off}, and compared the performance of the learned policies. \cref{fig:training_evoluation} shows the evolution of the AV average reward for two RL policies with (blue) and without (green) collision constraints. \BF{Until approximately 12$\times10^6$ steps, employing collision avoidance constraints limits the policy's exploration and thus, resulting in a slower increase on the average rewards. After, the \textit{Coll. On.} policy keeps improving, surpassing the \textit{Coll. Off.} in terms of average rewards. \cref{tab:ablation_coll_avd} presents the obtained performance results (i.e., percentage of successful episodes, collisions and timeouts). The policy trained with collision avoidance constraints (\textit{Coll. On}) achieves a higher success rate in all simulation settings. In contrast, not employing collision avoidance constraints (\textit{Coll. Off} policy) during training results in an overly conservative policy and, thus, in a significantly higher timeout rate.} %disables the AV to closely interact with other vehicles resulting in a more aggressive learned policy a higher collision rate. 

%disabling collision constraints during training and the policy's query frequency per number of $K$ control cycles on the training performance. Firstly, we have trained two policies using \cref{alg:training} with collision constraints, denoted by \textit{Coll. On}, and without collision constraints, denoted by \textit{Coll. Off}. We evaluated both policies for each cooperation setting (i.e., cooperative, mixed, and non-cooperative) 400 times, resulting in a total of 1200 evaluation episodes. Note that during evaluation, the collision avoidance constraints are enabled for both policies. \cref{tab:ablation_coll_avd} presents the obtained performance results. The policy trained without collision avoidance constraints (\textit{Coll. Off}) achieves a higher success rate in all simulation settings. In contrast, employing collision avoidance constraints (\textit{Coll. On} policy) during training disables the AV to closely interact with other vehicles resulting in a more aggressive learned policy a higher collision rate. 
